# Supplementary material for: Human Pose Regression with Residual Log-likelihood Estimation
Source: arXiv:2107.11291 source file (2021-07-31)
Supplement: Supplementary file 2 [file curve.tex]

\section{Training Curves}\label{sec:curve}
